# Supplementary material for: AdaptSR: Low-Rank Adaptation for Efficient and Scalable Real-World Super-Resolution
Source: arXiv:2503.07748 source file (2025-03-10)
Supplement: Supplementary file 1 [file X_suppl.tex]

% \clearpage
\setcounter{page}{1}
% \maketitlesupplementary

\section{Overview}
This document provides additional comparisons of fine-tuning and AdaptSR in terms of training efficiency, memory consumption and inference time in Section \ref{sec:adaptsr_ft_comparison}. Furthermore, we compare domain adaptation between baseline models and our LoRA-enhanced AdaptSR versions in Section \ref{sec:comp_domain_adapt}. Section \ref{sec:lwi_edsr} highlights the module-wise significance of low-rank adaptation for AdaptSR-C, a CNN-based architecture. %In Section \ref{sec:comb_lora_layers}, we explore how combining LoRA layers influences overall performance.
Lastly, Section \ref{sec:visuals_gan} offers visual comparisons between GAN approach and our AdaptSR-GAN for real SR, while Section \ref{sec:more_visuals} presents additional visual comparisons between our methods and the state-of-the-art GAN and diffusion models.

\section{AdaptSR vs. Fine-tuning Comparison}
\label{sec:adaptsr_ft_comparison}
Figure \ref{fig:lora_vs_ft} compares AdaptSR to full fine-tuning for bicubic-trained SR models. Fine-tuning updates all parameters, increasing memory usage and storage demands, while AdaptSR selectively updates lightweight LoRA layers for efficient adaptation. Full fine-tuning requires backpropagation through the entire network, leading to high GPU memory usage, especially for large transformer-based SR models. In contrast, AdaptSR reduces memory consumption by over 92\% by freezing the pretrained backbone. Additionally, AdaptSR merges LoRA updates post-training, introducing no inference cost. Storage-wise, full fine-tuning doubles model size, whereas AdaptSR only saves LoRA layers (e.g., 886k vs. 12M parameters), making it ideal for deployment on storage-constrained devices.

\begin{figure}
\centering
\includesvg[width=\linewidth]{images/lora_vs_ft2.svg}
\caption{\textbf{LoRA vs. FT:} Our efficient LoRA approach adapts SR models from bicubic to real-world degradations by updating only 8\% of parameters, avoiding the doubled storage requirements of full fine-tuning with no extra inference cost, while achieving comparable or superior performance on RealSR \cite{realsr_cai2019toward}.}
\label{fig:lora_vs_ft}
\end{figure}

\section{More Comparison for Domain Adaptation}
\label{sec:comp_domain_adapt}
Table \ref{table:domain_adaptation} shows additional comparisons between baseline models and our AdaptSR versions for domain adaptation from bicubic to real-world SR on DIV2K \cite{Agustsson_2017_CVPR_Workshops} and DRealSR \cite{drealsr_wei2020component}. Pretrained bicubic SR models exhibit notable performance drops when evaluated on unknown real-world images with complex degradations, representing their limited adaptability. Our LoRA-based method effectively addresses this gap, significantly enhancing performance on both datasets. Specifically, on the DIV2K validation set, our LoRA-enhanced models achieve up to 1 dB improvement in PSNR and a 25$\%$ reduction in LPIPS, reflecting both higher fidelity and perceptual quality. Similarly, on the challenging DRealSR dataset, LoRA adaptation boosts PSNR by 0.5 dB and reduces LPIPS by 20$\%$, despite not utilizing the DRealSR training set. This underscores the strong generalization capability of our approach, enabling it to adapt pretrained bicubic models to diverse real-world degradations effectively and efficiently.

\begin{figure*}[t!]
\centering
\includesvg[width=0.95\linewidth]{supp_visuals/adaptsr-c_arch}
\caption{Overview of AdaptSR-C, CNN based on EDSR \cite{EDSR2017} to adapt bicubic-trained SR models to real-world degradations. The deep feature extraction block includes 16 Residual LoRA Blocks (RLB). LoRA-modified convolutional reduce parameters and computational load, enabling efficient, high-resolution outputs.}
\label{fig:edsr_arch}
\end{figure*}

\begin{table*}
 \caption{Performance comparison for domain adaptation between bicubic-trained baseline models and LoRA-enhanced AdaptSR versions on realSR benchmarks \cite{Agustsson_2017_CVPR_Workshops, realsr_cai2019toward, drealsr_wei2020component}. LoRA substantially enhances validation results, achieving effective domain adaptation from bicubic to real SR with significantly fewer trainable parameters and reduced training time, while preserving the inference speed of the baseline models.}
    \centering
    \scalebox{0.9}{
    \begin{tabular}{lccccccccc}
    \specialrule{.1em}{.05em}{.05em} 
     & Metric & EDSR & AdaptSR-C & SAFMN & AdaptSR-T & SwinIR & AdaptSR & DRCT & AdaptSR-L \\ 
     \hline
   \multirow{4}{*}{DIV2K} & PSNR $\uparrow$ & 24.9164& 25.5393& 24.9298& 25.4742& 24.8738& \textbf{25.8058}& 24.8938& 25.7739 \\
    & SSIM $\uparrow$ &  0.6261& 0.6553& 0.6264& 0.6547& 0.6237& 0.6681& 0.6249& \textbf{0.6693} \\ 
    & LPIPS $\downarrow$ &  0.6740& 0.5376& 0.6758& 0.5461& 0.6731& 0.5047& 0.6744& \textbf{0.5037} \\
    & DISTS $\downarrow$ &  0.3304& 0.3324& 0.3308& 0.3271& 0.3305& 0.3194& 0.3301& \textbf{0.3167} \\ 
    \hline
    \multirow{4}{*}{RealSR} & PSNR $\uparrow$ & 27.5422 & 27.9322 & 27.5383 & 28.3216& 27.5537 & 28.7003 &27.5502 & \textbf{28.7245}\\
    & SSIM $\uparrow$ & 0.7732 & 0.7878 & 0.7740 & 0.7935 & 0.7738 & \textbf{0.8079} & 0.7737 & 0.8061 \\
   &  LPIPS $\downarrow$ & 0.3937 & 0.2835 & 0.3927 & 0.2935 & 0.3965 & 0.2591 & 0.3966 & \textbf{0.2553}\\
   &  DISTS $\downarrow$ &  0.2303 & 0.2190 & 0.2472 & 0.2291 & 0.2304 & 0.2109& 0.2584 & \textbf{0.2094} \\ 
    \hline
   \multirow{4}{*}{DRealSR} & PSNR $\uparrow$ & 30.6469& 30.6370& 30.6221& \textbf{30.9162}& 30.6209& 30.7392& 30.6066& 30.8109\\
    & SSIM $\uparrow$ &  0.8328& 0.8368& 0.8327& 0.8403& 0.8327& \textbf{0.8422}& 0.8325& 0.8419 \\
   &  LPIPS $\downarrow$ & 0.4364& 0.3523& 0.4356& 0.3529& 0.4391& \textbf{0.3381}& 0.4394& 0.3414\\
   &  DISTS $\downarrow$ &  0.2695& 0.2548& 0.2689& 0.2545& 0.2708& \textbf{0.2524}& 0.2703& 0.2544 \\ 
\specialrule{.1em}{.05em}{.05em} 
    \end{tabular} 
}
\label{table:domain_adaptation}
\end{table*}

\section{Module-wise Importance for AdaptSR-CNN}
\label{sec:lwi_edsr}
We also provide module-wise importance for AdaptSR-CNN using the baseline EDSR \cite{EDSR2017} architecture presented in Figure \ref{fig:edsr_arch} for domain adaptation from bicubic to real SR, we tested LoRA on four configurations: (1) first convolution layer (2) convolutional layers in Residual Blocks, (3) convolution layer before upsampling, and (4) convolution layer after upsampling. As presented in Table \ref{table:edsr_effect_of_lora_layers}, applying LoRA to all convolutional layers updating only 314k parameters of baseline model (1.5M) yield better fidelity and perceptual scores than individual convolutional layers. However, applying low-rank adaptation to convolutional layers either before upsampling (BU Conv) or after upsampling (AU Conv) yields better performance than adapting the initial convolutional layer (First Conv). Notably, these configurations achieve performance comparable to adapting convolutional layers within residual LoRA blocks (RLB Convs) while requiring significantly fewer parameter updates. Among these, the AU Conv layer stands out, providing optimal support for domain adaptation with an update of only 0.6k parameters.

\begin{table}
 \caption{\textit{Module-wise importance for LoRA domain adaptation} for AdaptSR-C architecture from bicubic to real SR on RealSR \cite{realsr_cai2019toward} dataset for rank 8.}
    \centering
    \scalebox{0.8}{
    \begin{tabular}{cccccl}
    \specialrule{.1em}{.05em}{.05em} 
    \multirow{2}{*}{LoRA Layer} & \multirow{2}{*}{PSNR} & \multirow{2}{*}{SSIM} & \multirow{2}{*}{LPIPS} & \multirow{2}{*}{DISTS} & Trainable  \\
    & & & & & Parameters \\ 
    \hline
   All Convs & \textbf{27.93} & \textbf{0.7878} & \textbf{0.2835} & \textbf{0.2190} & 314k \, (21$\%$)  \\
   \hdashline
   First Conv & 26.55 & 0.7473 &0.3773& 0.2552 & 4.8k \, (0.3$\%$)  \\
   RLB Convs & 27.54 & 0.7741 & 0.3935& 0.2438 & 295k \, (20$\%$) \\
   BU Conv & 27.54 & 0.7740 & 0.3941& 0.2437 & 9.2k \, (0.6$\%$) \\
   AU Conv & 27.54 & 0.7740 & 0.3937& 0.2436 & 4.8k \, (0.6$\%$) \\
\specialrule{.1em}{.05em}{.05em} 
    \end{tabular} 
}
\label{table:edsr_effect_of_lora_layers}
\end{table}

% \section{Combination of LoRA Layers}
% \label{sec:comb_lora_layers}
% We further analize the effect of combinational LoRA layers and present them in Table \ref{table:supp_effect_of_lora_layers} while adapting SwinIR \cite{liang2021swinir} to real SR. 

\section{Rank Analysis for Other Baselines}

\textbf{Scaling Factor.}
\label{sec:scaling}
The scaling factor in AdaptSR plays a crucial role in balancing adaptation strength and stability during domain adaptation. As shown in Table \ref{table:scaling_ablation}, reducing the scaling factor from 1 to 0.125 consistently improves PSNR, SSIM, and perceptual metrics, indicating more effective adaptation to real-world degradations. Notably, a scaling factor of 0.125 achieves the best overall performance, suggesting that smaller updates help fine-tune the model without overfitting to specific degradations. However, an excessively low scaling factor (0.0625) leads to a sharp drop in PSNR and perceptual quality, likely due to insufficient adaptation capacity. These results highlight the importance of carefully selecting the scaling factor to optimize performance while maintaining stability in real SR adaptation.

\begin{table}
 \caption{Ablation on scaling factor on RealSR \cite{realsr_cai2019toward} for AdaptSR.} 
    \centering
    \scalebox{0.95}{
    \begin{tabular}{lcccc}
    \specialrule{.1em}{.05em}{.05em} 
    Scaling Factor & PSNR & SSIM & LPIPS & DISTS \\
    \hline
    1 & 27.6252& 0.7767& 0.3917& 0.2430 \\
    0.5 & 27.6684& 0.7780& 0.3825& 0.2414\\
    0.25 & 27.7357& 0.7801& 0.3688& 0.2395\\
    0.125 & \textbf{28.7023} & \textbf{0.8079}& \textbf{0.2591} & \textbf{0.2109}\\
    0.0625 & 22.6364& 0.6357& 0.4246& 0.3066 \\
\specialrule{.1em}{.05em}{.05em} 
    \end{tabular} 
}
\label{table:scaling_ablation}
\end{table}

\section{Visual Results for GAN-Based LoRA}
\label{sec:visuals_gan}
We present additional visual comparisons with state-of-the-art GAN method (LDL \cite{liang2022details}) and our LoRA-based GAN method in Figure \ref{fig:gan_results}. It is worth mentioning that both architectures use the same generator architecture \cite{liang2021swinir} and in our adaptation approach we only injected LoRA layers to the same generator. Figure \ref{fig:gan_results} shows that the proposed approach can further extend to adversarial training and provides clearer images with fine detailed structures than GAN method.

\begin{figure}
\centering
\begin{subfigure}{0.14\textwidth}
     \begin{subfigure}{\textwidth}
        \includegraphics[width=\textwidth]{supp_visuals/Nikon_041hr.pdf} 
    \end{subfigure}
    \caption*{Nikon 41- HR \\ PSNR/SSIM}
\end{subfigure}
\begin{subfigure}{0.14\textwidth}
     \begin{subfigure}{\textwidth}
        \includegraphics[width=\textwidth]{supp_visuals/Nikon_041ldl_swinir.pdf} 
    \end{subfigure}
    \caption*{LDL \cite{liang2022details} \\  16.446 / 0.738}
\end{subfigure}
\begin{subfigure}{0.14\textwidth}
     \begin{subfigure}{\textwidth}
        \includegraphics[width=\textwidth]{supp_visuals/Nikon_041ours_gan.pdf}
    \end{subfigure}
    \caption*{AdaptSR-GAN \\ 17.799 / 0.880
}
\end{subfigure}
\begin{subfigure}{0.14\textwidth}
    \begin{subfigure}{\textwidth}
        \includegraphics[width=\textwidth]{supp_visuals/Nikon_050hr.pdf} 
    \end{subfigure}
\caption*{Nikon 50- HR\\ PSNR/SSIM}
\end{subfigure}
\begin{subfigure}{0.14\textwidth}
    \begin{subfigure}{\textwidth}
        \includegraphics[width=\textwidth]{supp_visuals/Nikon_050ldl_swinir.pdf} 
    \end{subfigure}
\caption*{LDL \cite{liang2022details} \\ 20.879 / 0.956}
\end{subfigure}
\begin{subfigure}{0.14\textwidth}
    \begin{subfigure}{\textwidth}
        \includegraphics[width=\textwidth]{supp_visuals/Nikon_050ours_gan.pdf} 
    \end{subfigure}
\caption*{AdaptSR-GAN \\ 25.615 / 0.981}
\end{subfigure}
\begin{subfigure}{0.14\textwidth}
    \begin{subfigure}{\textwidth}
        \includegraphics[width=\textwidth]{supp_visuals/Canon_004hr.pdf} 
    \end{subfigure}
\caption*{Canon 04- HR\\ PSNR/SSIM}
\end{subfigure}
\begin{subfigure}{0.14\textwidth}
    \begin{subfigure}{\textwidth}
        \includegraphics[width=\textwidth]{supp_visuals/Canon_004ldl_swinir.pdf} 
    \end{subfigure}
\caption*{LDL \cite{liang2022details} \\ 22.646 / 0.904}
\end{subfigure}
\begin{subfigure}{0.14\textwidth}
    \begin{subfigure}{\textwidth}
        \includegraphics[width=\textwidth]{supp_visuals/Canon_004ours_gan.pdf} 
    \end{subfigure}
\caption*{AdaptSR-GAN \\ 27.877 / 0.980}
\end{subfigure}
\caption{Visual results for GAN-based real SR methods on RealSR \cite{realsr_cai2019toward} dataset. The proposed model with adversarial training reconstructs better images.} 
\label{fig:gan_results} 
\end{figure}

\section{More Visual Results}
\label{sec:more_visuals}

We provide further visual comparisons of $\times$4 Real SR results between our proposed AdaptSR method and the other state-of-the-art GAN and diffusion methods including LDL \cite{liang2022details}, Real-SAFMN-L \cite{safmn_sun2023spatially}, PASD \cite{yang2023pasd} and OSEDiff \cite{lora_diff_realsr_wu2024one} in Figure \ref{fig:qual_results_supp} to Figure \ref{fig:qual_results_supp2}. From these visual comparisons, one can draw consistent observations in line with the results in the paper. GAN models, LDL \cite{liang2022details} and SAFMN-Large \cite{safmn_sun2023spatially}, often introduce artifacts, such as blending the man’s nose with the background or failing to reproduce textures. Similarly, diffusion-based methods, PASD \cite{yang2023pasd} and OSEDiff \cite{lora_diff_realsr_wu2024one} exhibit excessive sharpness with content inaccuracies, omitting details like the man’s mustache or failing to recover textures. In contrast, our LoRA-based models adeptly reconstruct high-fidelity details, particularly in complex areas with regular patterns, such as retaining the man’s mustache and restoring textures to match the HR image. Overall, our LoRA-based approaches not only suppresses visual artifacts but also simultaneously restores structural shapes and realistic details.

\begin{figure*}[t!]
\centering
\begin{subfigure}{0.295\textwidth}
     \begin{subfigure}{\textwidth}
        \includegraphics[width=\textwidth]{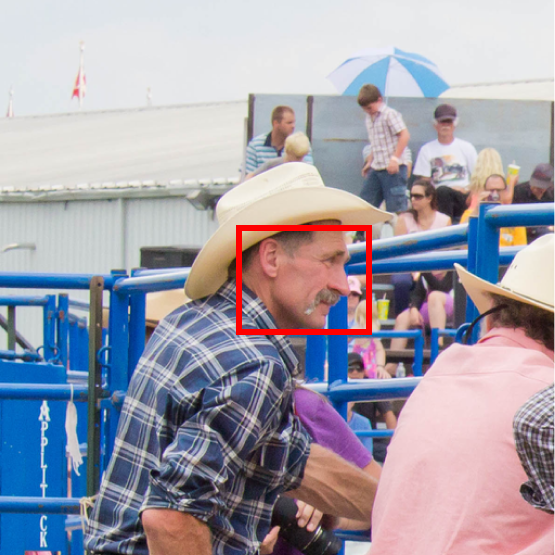} \vspace{-8pt}\\ \centering \scriptsize DIV2K \cite{Agustsson_2017_CVPR_Workshops} \\ 804 (patch 00001)
    \end{subfigure}
         \begin{subfigure}{\textwidth}
        \includegraphics[width=\textwidth]{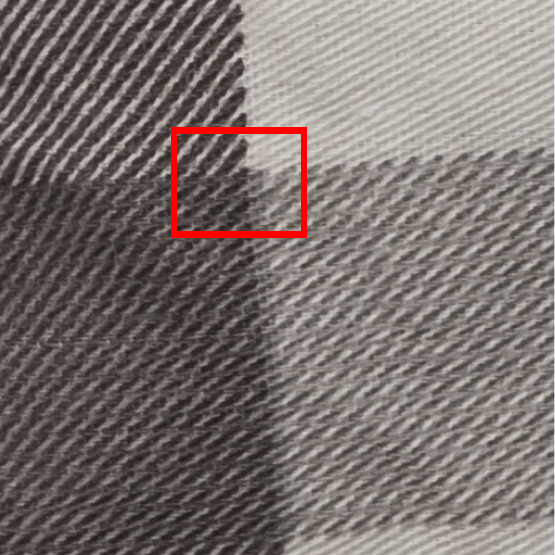} \vspace{-8pt}\\ \centering \scriptsize RealSR \cite{realsr_cai2019toward} \\ Nikon 21 
    \end{subfigure}
         \begin{subfigure}{\textwidth}
        \includegraphics[width=\textwidth]{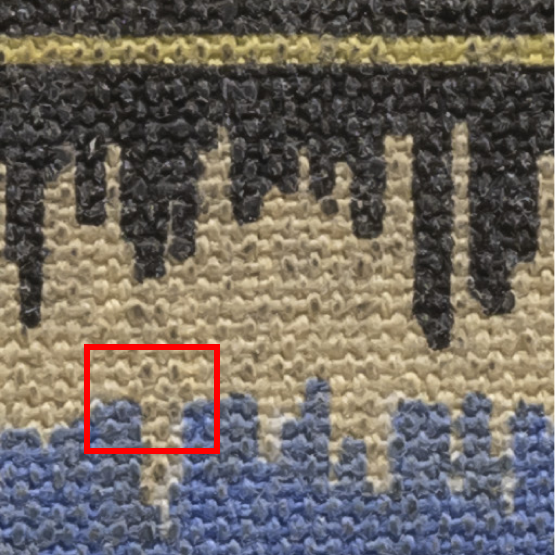} \vspace{-8pt}\\ \centering \scriptsize RealSR \cite{realsr_cai2019toward} \\ Nikon 27  
    \end{subfigure}
\end{subfigure}
\begin{subfigure}{0.16\textwidth}
    \begin{subfigure}{\textwidth}
        \includegraphics[width=\textwidth]{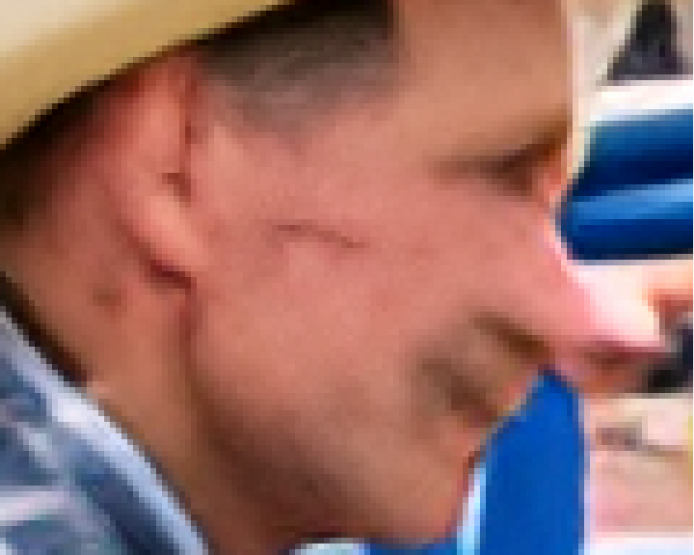}
        \vspace{-8pt}\\ \centering \scriptsize LDL \cite{liang2022details} \\ (23.095/0.939)
    \end{subfigure}
    \begin{subfigure}{\textwidth}
        \includegraphics[width=\textwidth]{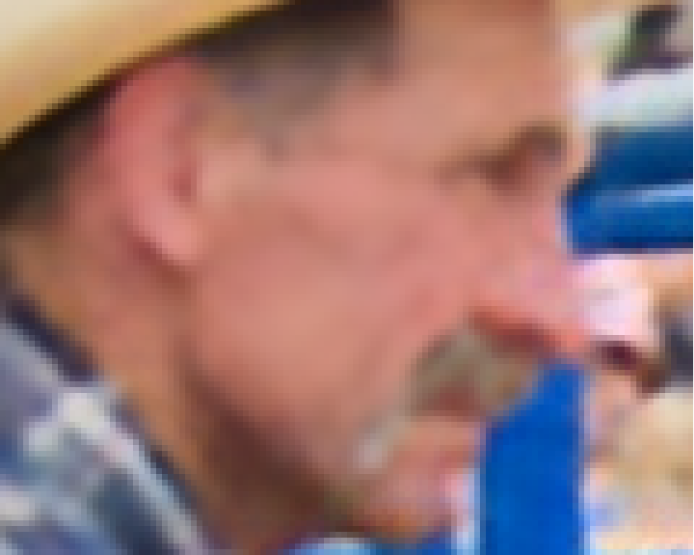} \vspace{-8pt}\\ \centering \scriptsize AdaptSR-T \\ (27.791/0.963)
    \end{subfigure}
        \begin{subfigure}{\textwidth}
        \includegraphics[width=\textwidth]{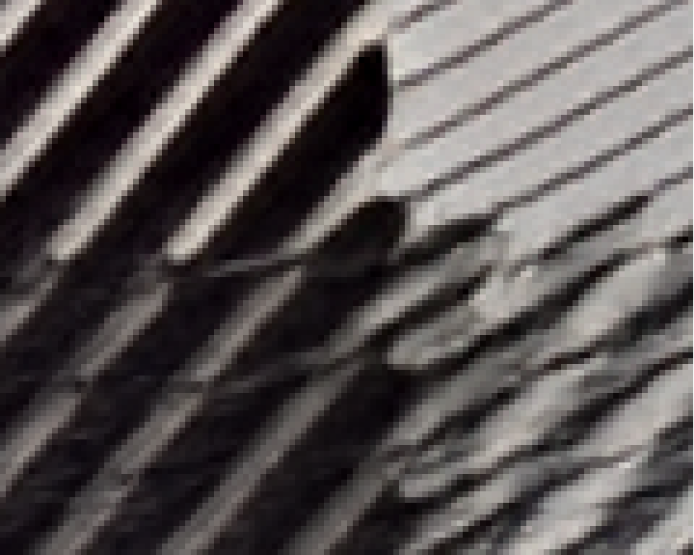}
        \vspace{-8pt}\\ \centering \scriptsize LDL \cite{liang2022details} \\ (17.166/0.804)
    \end{subfigure}
    \begin{subfigure}{\textwidth}
        \includegraphics[width=\textwidth]{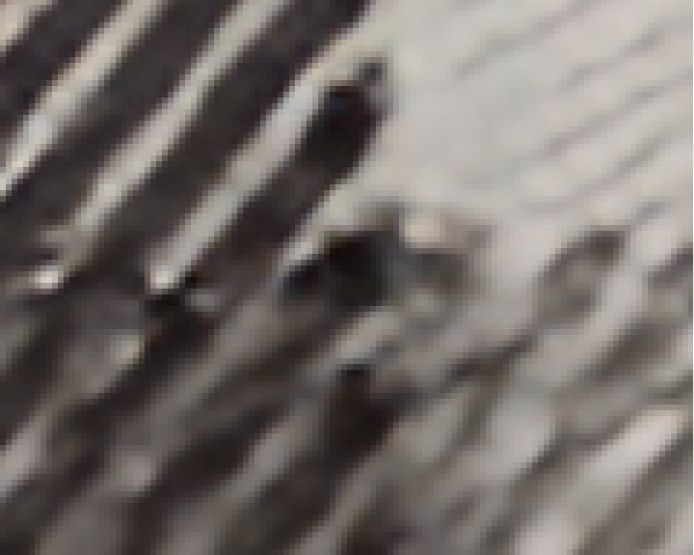} \vspace{-8pt}\\ \centering \scriptsize AdaptSR-T \\ (21.010/0.914)
    \end{subfigure}
    \begin{subfigure}{\textwidth}
        \includegraphics[width=\textwidth]{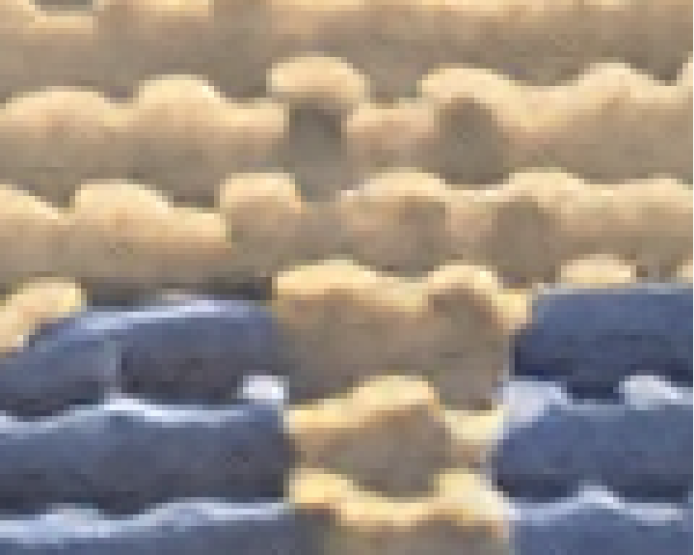}
        \vspace{-8pt}\\ \centering \scriptsize LDL \cite{liang2022details} \\ (21.355/0.928)
    \end{subfigure}
    \begin{subfigure}{\textwidth}
        \includegraphics[width=\textwidth]{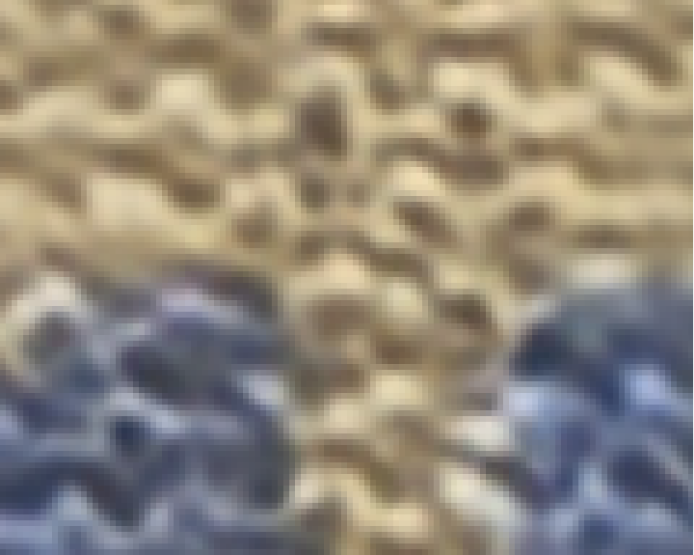} \vspace{-8pt}\\ \centering \scriptsize AdaptSR-T \\ (26.613/0.960)
    \end{subfigure}
\end{subfigure}
\begin{subfigure}{0.16\textwidth}
    \begin{subfigure}{\textwidth}
        \includegraphics[width=\textwidth]{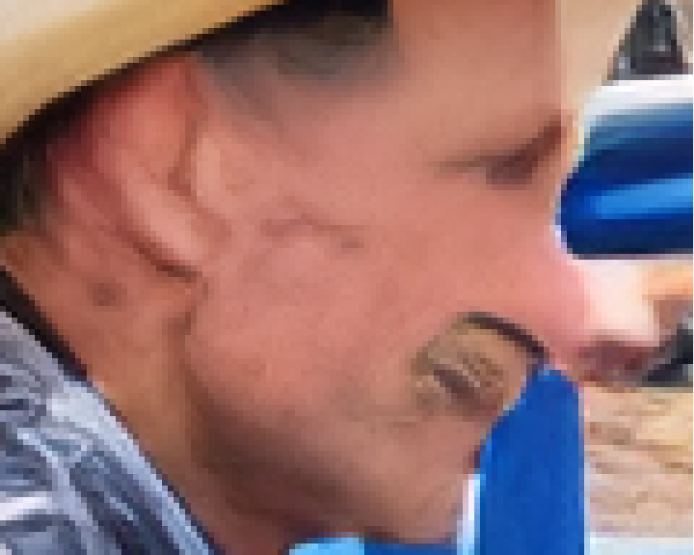} \vspace{-8pt}\\\centering \scriptsize  Real SAFMN-L \cite{safmn_sun2023spatially} \\ (23.807/0.939)
    \end{subfigure}
    \begin{subfigure}{\textwidth}
        \includegraphics[width=\textwidth]{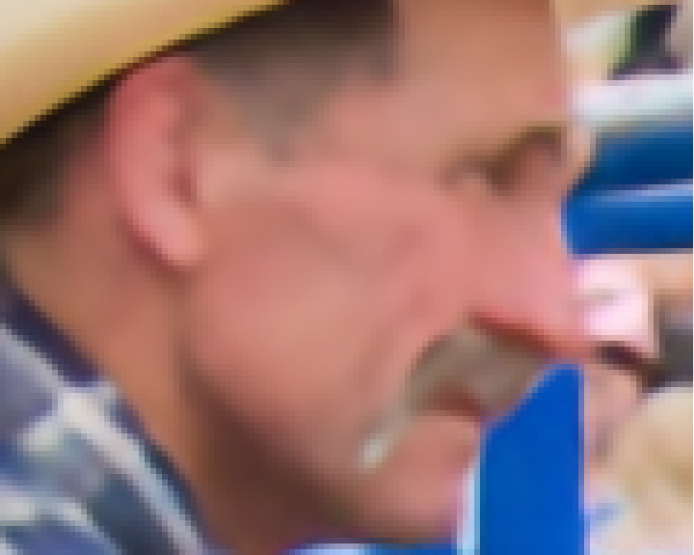} \vspace{-8pt}\\ \centering \scriptsize AdaptSR \\ (28.750/0.967)
    \end{subfigure}
        \begin{subfigure}{\textwidth}
        \includegraphics[width=\textwidth]{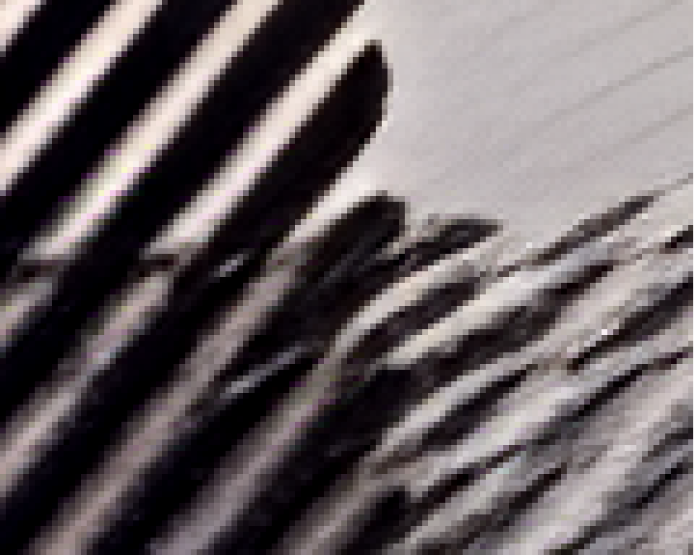} \vspace{-8pt}\\\centering \scriptsize  Real SAFMN-L \cite{safmn_sun2023spatially} \\ (15.837/0.755)
    \end{subfigure}
    \begin{subfigure}{\textwidth}
        \includegraphics[width=\textwidth]{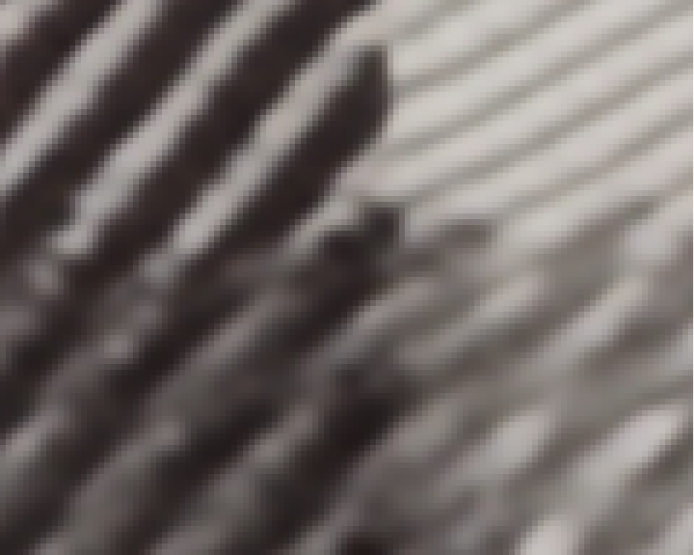} \vspace{-8pt}\\ \centering \scriptsize AdaptSR \\ (23.902/0.943)
    \end{subfigure}
        \begin{subfigure}{\textwidth}
        \includegraphics[width=\textwidth]{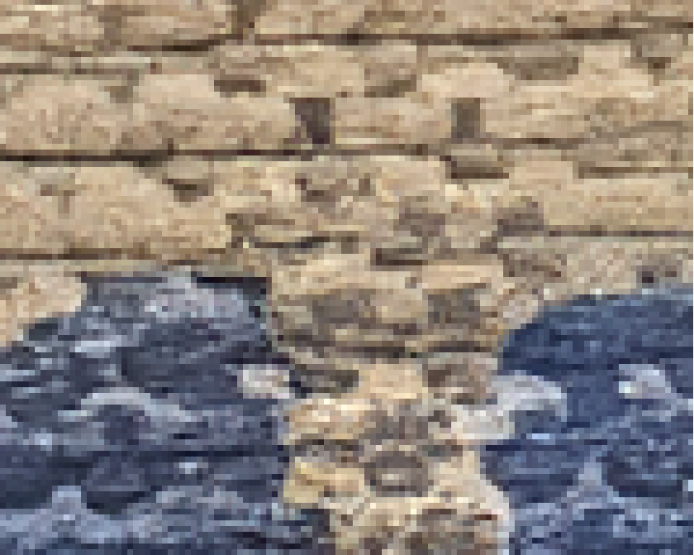} \vspace{-8pt}\\\centering \scriptsize  Real SAFMN-L \cite{safmn_sun2023spatially} \\ (18.836/0.837)
    \end{subfigure}
    \begin{subfigure}{\textwidth}
        \includegraphics[width=\textwidth]{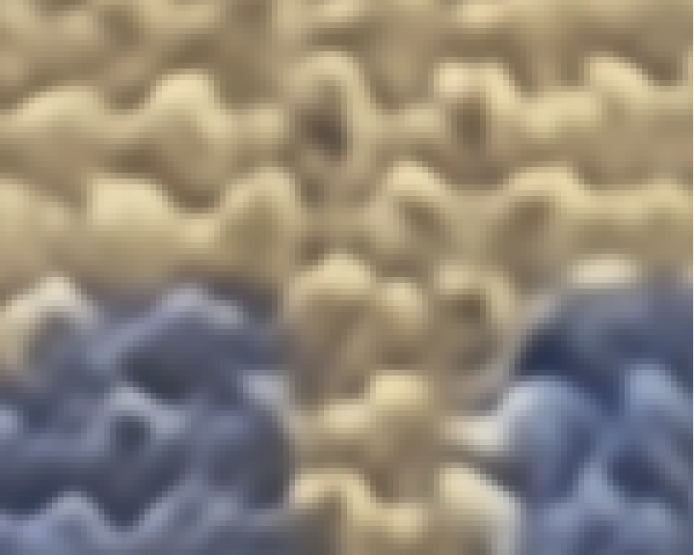} \vspace{-8pt}\\ \centering \scriptsize AdaptSR \\ (28.042/0.967)
    \end{subfigure}
\end{subfigure}
\begin{subfigure}{0.16\textwidth}
    \begin{subfigure}{\textwidth}
        \includegraphics[width=\textwidth]{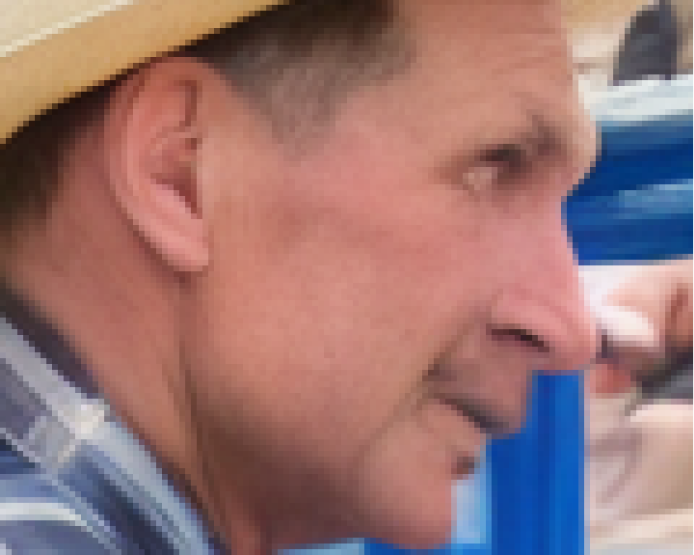} \vspace{-8pt}\\\centering \scriptsize PASD \cite{yang2023pasd} \\ (24.489/0.945)
    \end{subfigure}
    \begin{subfigure}{\textwidth}
        \includegraphics[width=\textwidth]{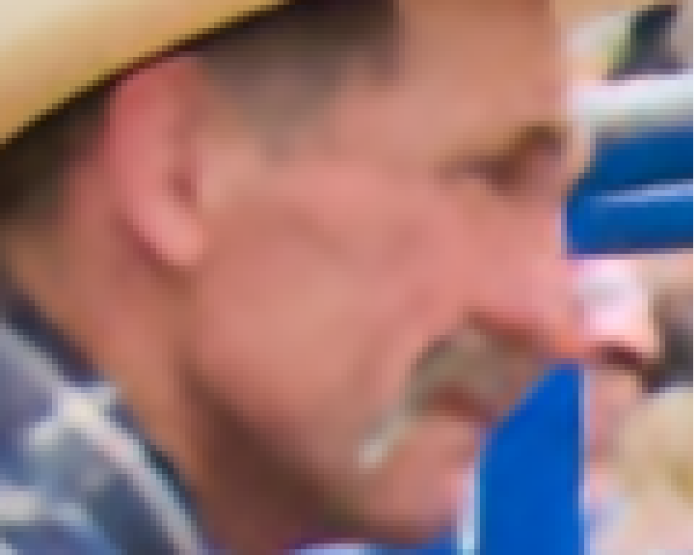} \vspace{-8pt}\\ \centering \scriptsize AdaptSR-L \\ (28.356/0.966)
    \end{subfigure}
        \begin{subfigure}{\textwidth}
        \includegraphics[width=\textwidth]{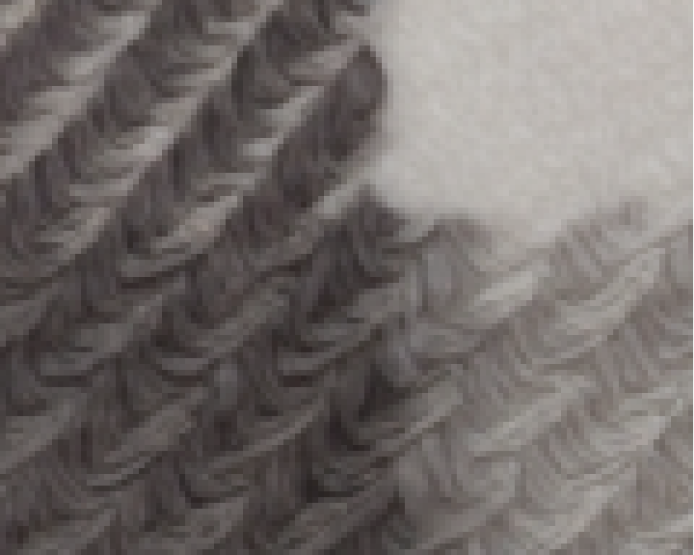} \vspace{-8pt}\\\centering \scriptsize PASD \cite{yang2023pasd} \\ (22.673/0.922)
    \end{subfigure}
    \begin{subfigure}{\textwidth}
        \includegraphics[width=\textwidth]{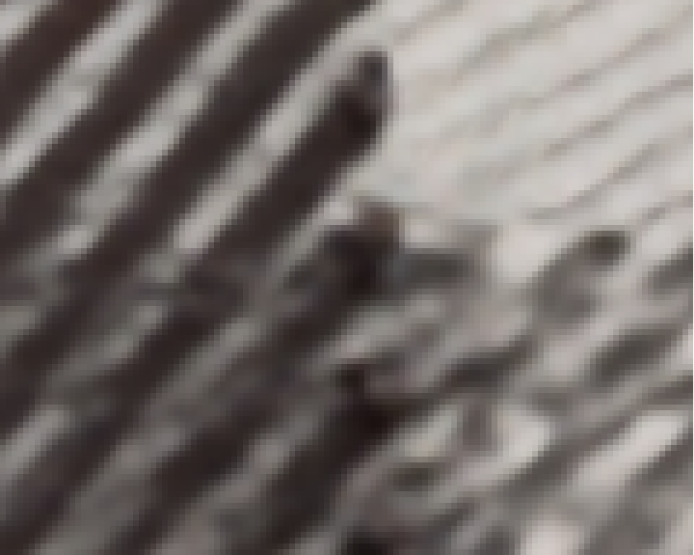} \vspace{-8pt}\\ \centering \scriptsize AdaptSR-L \\ (21.332/0.921)
    \end{subfigure}
            \begin{subfigure}{\textwidth}
        \includegraphics[width=\textwidth]{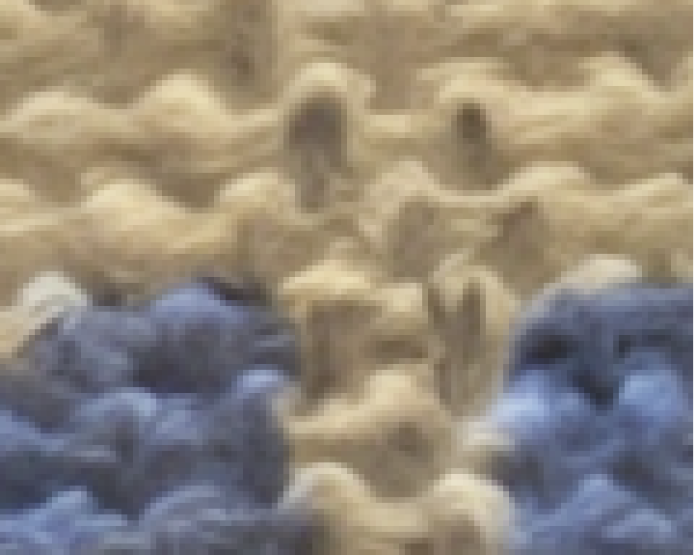} \vspace{-8pt}\\\centering \scriptsize PASD \cite{} \\ (25.013/0.943)
    \end{subfigure}
    \begin{subfigure}{\textwidth}
        \includegraphics[width=\textwidth]{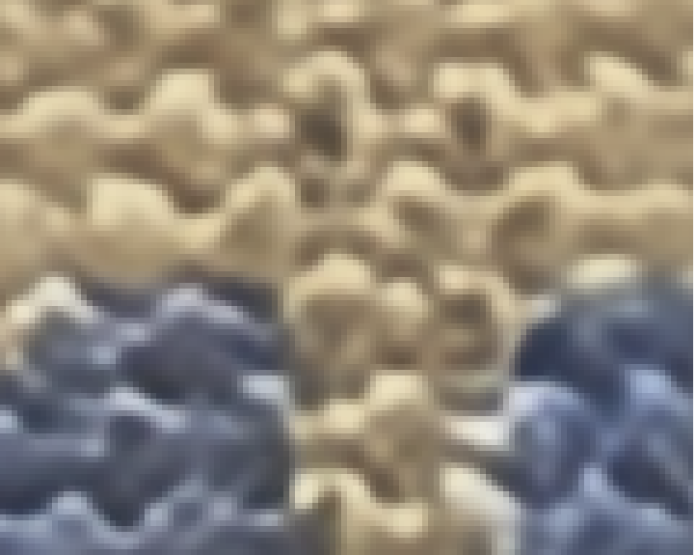} \vspace{-8pt}\\ \centering \scriptsize AdaptSR-L \\ (26.315/0.960)
    \end{subfigure}
\end{subfigure}
\begin{subfigure}{0.16\textwidth}
    \begin{subfigure}{\textwidth}
        \includegraphics[width=\textwidth]{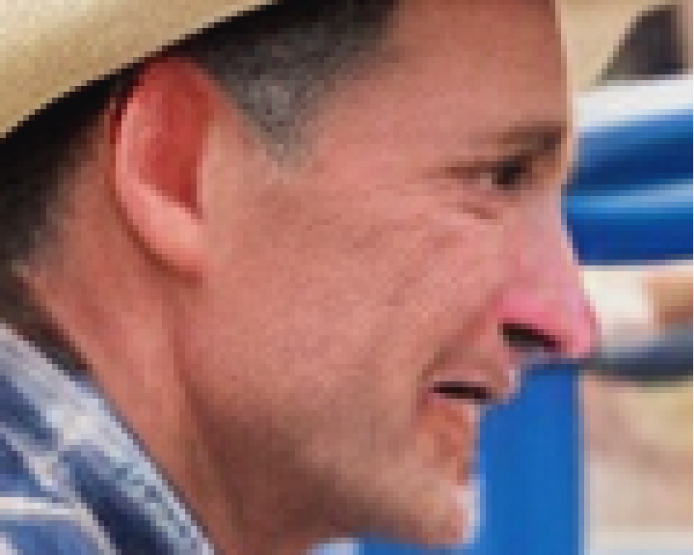} \vspace{-8pt}\\ \centering \scriptsize OSEDiff \cite{lora_diff_realsr_wu2024one} \\ (22.600/0.933)
    \end{subfigure}
     \begin{subfigure}{\textwidth}
        \includegraphics[width=\textwidth]{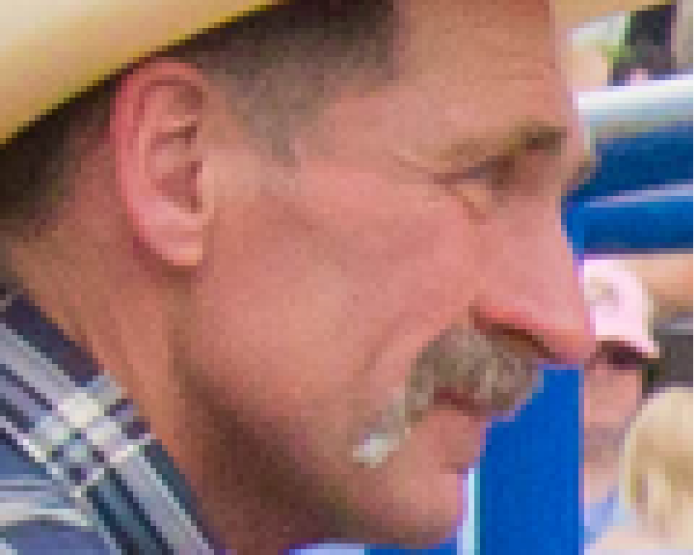} \vspace{-8pt}\\ \centering \scriptsize HR Crop \\  (PSNR/SSIM)
    \end{subfigure}
    \begin{subfigure}{\textwidth}
        \includegraphics[width=\textwidth]{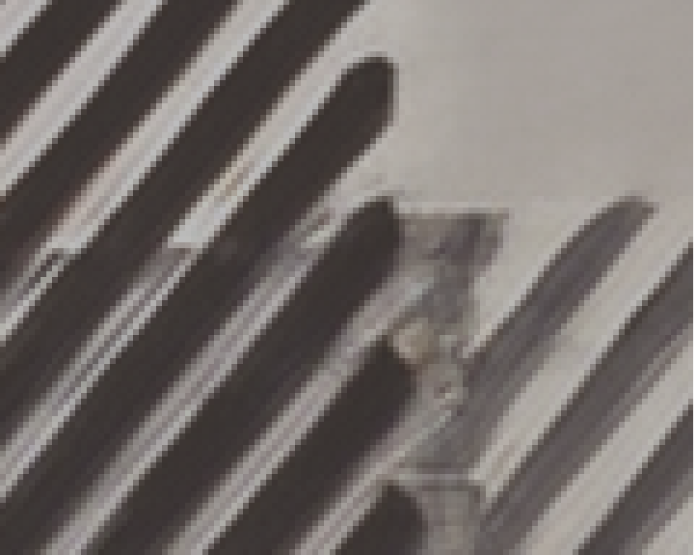} \vspace{-8pt}\\ \centering \scriptsize OSEDiff \cite{lora_diff_realsr_wu2024one} \\ (20.402/0.910)
    \end{subfigure}
     \begin{subfigure}{\textwidth}
        \includegraphics[width=\textwidth]{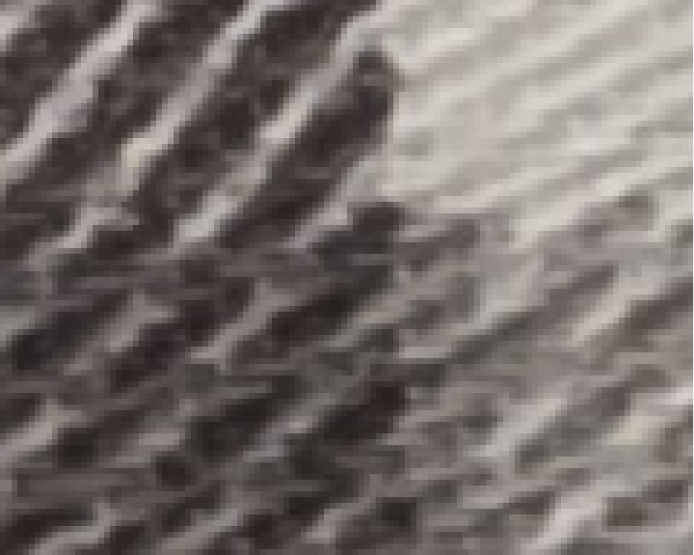} \vspace{-8pt}\\ \centering \scriptsize HR Crop  \\  (PSNR/SSIM)
    \end{subfigure}
    \begin{subfigure}{\textwidth}
        \includegraphics[width=\textwidth]{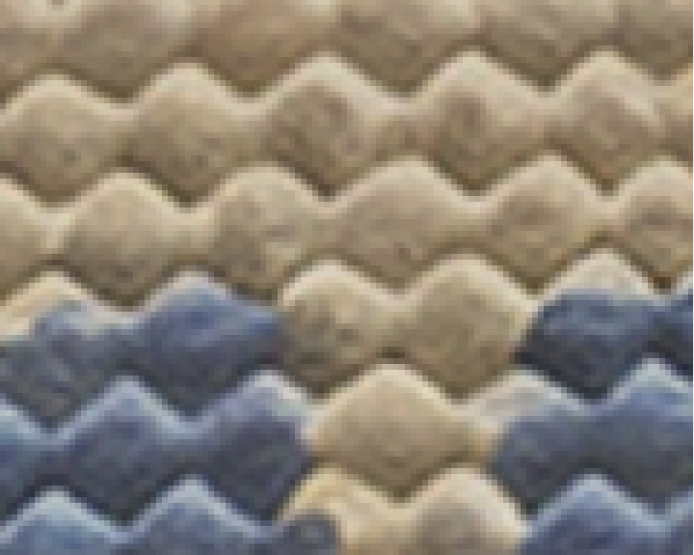} \vspace{-8pt}\\ \centering \scriptsize OSEDiff \cite{lora_diff_realsr_wu2024one} \\ (20.802/0.914)
    \end{subfigure}
     \begin{subfigure}{\textwidth}
        \includegraphics[width=\textwidth]{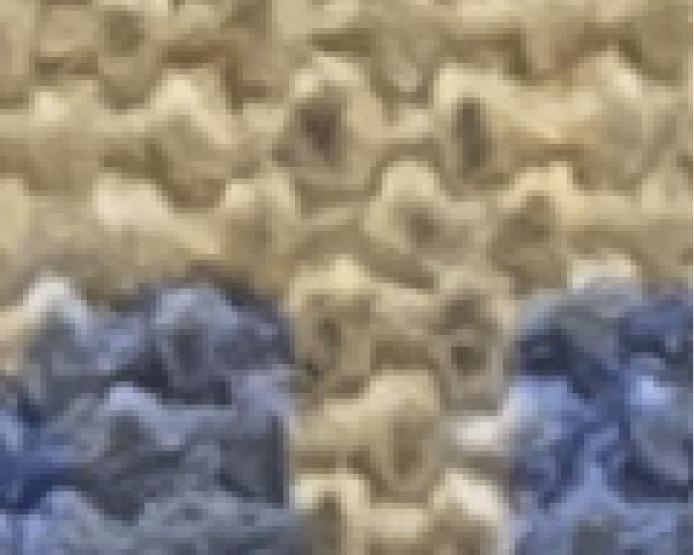} \vspace{-8pt}\\ \centering \scriptsize HR Crop  \\  (PSNR/SSIM)
    \end{subfigure}
\end{subfigure}
\vspace{-3pt}
\caption{Visual comparison of the proposed LoRA-enhanced models (AdaptSR and its variants) with the state-of-the-art methods for $\times$4 real SR. GAN and diffusion models fail to capture the correct content of images, however, our AdaptSR models reconstruct high-fidelity and realistic details with correct alignment.}
\label{fig:qual_results_supp} 
\end{figure*}

\begin{figure*}[t!]
\centering
\begin{subfigure}{0.295\textwidth}
     \begin{subfigure}{\textwidth}
        \includegraphics[width=\textwidth]{supp_visuals/0861_pch_00010hr_with_rectangle.pdf} \vspace{-8pt}\\ \centering \scriptsize DIV2K \cite{Agustsson_2017_CVPR_Workshops} \\ 861 (patch 00010)
    \end{subfigure}
         \begin{subfigure}{\textwidth}
        \includegraphics[width=\textwidth]{supp_visuals/Canon_018hr_with_rectangle.pdf} \vspace{-8pt}\\ \centering \scriptsize RealSR \cite{realsr_cai2019toward} \\ Canon 18  
    \end{subfigure}
         \begin{subfigure}{\textwidth}
        \includegraphics[width=\textwidth]{supp_visuals/Canon_027hr_with_rectangle.pdf} \vspace{-8pt}\\ \centering \scriptsize RealSR \cite{realsr_cai2019toward} \\ Canon 27  
    \end{subfigure}
\end{subfigure}
\begin{subfigure}{0.16\textwidth}
    \begin{subfigure}{\textwidth}
        \includegraphics[width=\textwidth]{supp_visuals/0861_pch_00010ldl_swinir.pdf}
        \vspace{-8pt}\\ \centering \scriptsize LDL \cite{liang2022details} \\ (18.200/0.893)
    \end{subfigure}
    \begin{subfigure}{\textwidth}
        \includegraphics[width=\textwidth]{supp_visuals/0861_pch_00010safmn_lora.pdf} \vspace{-8pt}\\ \centering \scriptsize AdaptSR-T \\ (22.489/0.917)
    \end{subfigure}
        \begin{subfigure}{\textwidth}
        \includegraphics[width=\textwidth]{supp_visuals/Canon_018ldl_swinir.pdf}
        \vspace{-8pt}\\ \centering \scriptsize LDL \cite{liang2022details} \\ (25.272/0.964)
    \end{subfigure}
    \begin{subfigure}{\textwidth}
        \includegraphics[width=\textwidth]{supp_visuals/Canon_018safmn_lora.pdf} \vspace{-8pt}\\ \centering \scriptsize AdaptSR-T \\ (29.770/0.983)
    \end{subfigure}
    \begin{subfigure}{\textwidth}
        \includegraphics[width=\textwidth]{supp_visuals/Canon_027ldl_swinir.pdf}
        \vspace{-8pt}\\ \centering \scriptsize LDL \cite{liang2022details} \\ (20.870/0.923)   
    \end{subfigure}
    \begin{subfigure}{\textwidth}
        \includegraphics[width=\textwidth]{supp_visuals/Canon_027safmn_lora.pdf} \vspace{-8pt}\\ \centering \scriptsize AdaptSR-T \\ (22.607/0.943)
    \end{subfigure}
\end{subfigure}
\begin{subfigure}{0.16\textwidth}
    \begin{subfigure}{\textwidth}
        \includegraphics[width=\textwidth]{supp_visuals/0861_pch_00010safmn.pdf} \vspace{-8pt}\\\centering \scriptsize  Real SAFMN-L \cite{safmn_sun2023spatially} \\ (19.363/0.892)
    \end{subfigure}
    \begin{subfigure}{\textwidth}
        \includegraphics[width=\textwidth]{supp_visuals/0861_pch_00010swinir_lora.pdf} \vspace{-8pt}\\ \centering \scriptsize AdaptSR \\ (22.904/0.922)
    \end{subfigure}
        \begin{subfigure}{\textwidth}
        \includegraphics[width=\textwidth]{supp_visuals/Canon_018safmn.pdf} \vspace{-8pt}\\\centering \scriptsize  Real SAFMN-L \cite{safmn_sun2023spatially} \\ (24.777/0.964)
    \end{subfigure}
    \begin{subfigure}{\textwidth}
        \includegraphics[width=\textwidth]{supp_visuals/Canon_018swinir_lora.pdf} \vspace{-8pt}\\ \centering \scriptsize AdaptSR \\ (29.274/0.981)
    \end{subfigure}
        \begin{subfigure}{\textwidth}
        \includegraphics[width=\textwidth]{supp_visuals/Canon_027safmn.pdf} \vspace{-8pt}\\\centering \scriptsize  Real SAFMN-L \cite{safmn_sun2023spatially} \\ (20.491/0.914)
    \end{subfigure}
    \begin{subfigure}{\textwidth}
        \includegraphics[width=\textwidth]{supp_visuals/Canon_027swinir_lora.pdf} \vspace{-8pt}\\ \centering \scriptsize AdaptSR \\ (22.963/0.944)
    \end{subfigure}
\end{subfigure}
\begin{subfigure}{0.16\textwidth}
    \begin{subfigure}{\textwidth}
        \includegraphics[width=\textwidth]{supp_visuals/0861_pch_00010pasd.pdf} \vspace{-8pt}\\\centering \scriptsize PASD \cite{yang2023pasd} \\ (19.733/0.896)
    \end{subfigure}
    \begin{subfigure}{\textwidth}
        \includegraphics[width=\textwidth]{supp_visuals/0861_pch_00010drct_lora.pdf} \vspace{-8pt}\\ \centering \scriptsize AdaptSR-L \\ (22.815/0.921)
    \end{subfigure}
        \begin{subfigure}{\textwidth}
        \includegraphics[width=\textwidth]{supp_visuals/Canon_018pasd.pdf} \vspace{-8pt}\\\centering \scriptsize PASD \cite{yang2023pasd} \\ (27.368/0.966)
    \end{subfigure}
    \begin{subfigure}{\textwidth}
        \includegraphics[width=\textwidth]{supp_visuals/Canon_018drct_lora.pdf} \vspace{-8pt}\\ \centering \scriptsize AdaptSR-L \\ (29.793/0.982)
    \end{subfigure}
            \begin{subfigure}{\textwidth}
        \includegraphics[width=\textwidth]{supp_visuals/Canon_027pasd.pdf} \vspace{-8pt}\\\centering \scriptsize PASD \cite{yang2023pasd} \\ (21.321/0.924)

    \end{subfigure}
    \begin{subfigure}{\textwidth}
        \includegraphics[width=\textwidth]{supp_visuals/Canon_027drct_lora.pdf} \vspace{-8pt}\\ \centering \scriptsize AdaptSR-L \\ (22.913/0.945)
    \end{subfigure}
\end{subfigure}
\begin{subfigure}{0.16\textwidth}
    \begin{subfigure}{\textwidth}
        \includegraphics[width=\textwidth]{supp_visuals/0861_pch_00010osediff.pdf} \vspace{-8pt}\\ \centering \scriptsize OSEDiff \cite{lora_diff_realsr_wu2024one} \\ (19.157/0.898)
    \end{subfigure}
     \begin{subfigure}{\textwidth}
        \includegraphics[width=\textwidth]{supp_visuals/0861_pch_00010hr_crop.pdf} \vspace{-8pt}\\ \centering \scriptsize HR Crop \\  (PSNR/SSIM)
    \end{subfigure}
    \begin{subfigure}{\textwidth}
        \includegraphics[width=\textwidth]{supp_visuals/Canon_018osediff.pdf} \vspace{-8pt}\\ \centering \scriptsize OSEDiff \cite{lora_diff_realsr_wu2024one} \\ (24.126/0.958)
    \end{subfigure}
     \begin{subfigure}{\textwidth}
        \includegraphics[width=\textwidth]{supp_visuals/Canon_018hr_crop.pdf} \vspace{-8pt}\\ \centering \scriptsize HR Crop  \\  (PSNR/SSIM)
    \end{subfigure}
    \begin{subfigure}{\textwidth}
        \includegraphics[width=\textwidth]{supp_visuals/Canon_027osediff.pdf} \vspace{-8pt}\\ \centering \scriptsize OSEDiff \cite{lora_diff_realsr_wu2024one} \\ (21.182/0.925)
    \end{subfigure}
     \begin{subfigure}{\textwidth}
        \includegraphics[width=\textwidth]{supp_visuals/Canon_027hr_crop.pdf} \vspace{-8pt}\\ \centering \scriptsize HR Crop  \\  (PSNR/SSIM)
    \end{subfigure}
\end{subfigure}
\caption{Visual comparison of the proposed LoRA-enhanced models (AdaptSR and its variants) with the state-of-the-art methods for $\times$4 real SR. GAN and diffusion models fail to capture the correct content of images, however, our AdaptSR models reconstruct high-fidelity and realistic details with correct alignment.}
\label{fig:qual_results_supp2} 
\end{figure*}
